# Supplementary material for: A First Look at On-device Models in iOS Apps
Source: arXiv:2307.12328 source file (2023-07-27)
Supplement: Supplementary file 1 [file appendix.tex]

\section{Appendix}

\subsection{Adversarial Attack}
The whole process of adversarial attacking can be summarized as
\begin{equation}
    x^{'}_{adv} = x + \epsilon * attack_i(\nabla J (\theta,\ x,\ y_{true}))
\end{equation}
where $y_{true}$ represents the original label or class of input image $x$, $\epsilon$ represents a multiplier to ensure the perturbations between input images to adversarial images are small and its value is empirically determined in the experiments to produce unnoticeable image perturbations, $attack_i$ represents the $i_{th}$ type of adversarial attack, $\theta$ represents parameters, and $J$ is the loss.

\subsection{Examples of attacking real-world iOS apps}
\label{sec:realworld}
Figure~\ref{fig:phAt1} shows the attack results of the app \emph{gradient: celebrity look alike}.
The adversarial example image can directly cause the app to misclassify the gender of the image from male to female.

Figure~\ref{fig:phAt2} shows the attack results of the app \emph{smart bird id}.
The adversarial example image can directly cause the app to misclassify the bird type of the image from \emph{Australia Magpie} to \emph{Satin Bowerbird}.

\begin{figure}[htb]
    \centering
    \includegraphics[width=0.7\linewidth]{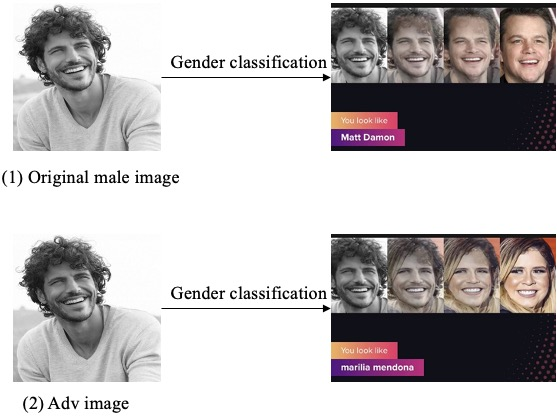}
    \caption{Example of attacking the feature of gender classification in the real-world app \emph{gradient: celebrity look alike}. The \emph{Adv image} is generated by attacking the corresponding model on Android}
    \label{fig:phAt1}
\end{figure}

\begin{figure}[htb]
    \centering
    \includegraphics[width=0.7\linewidth]{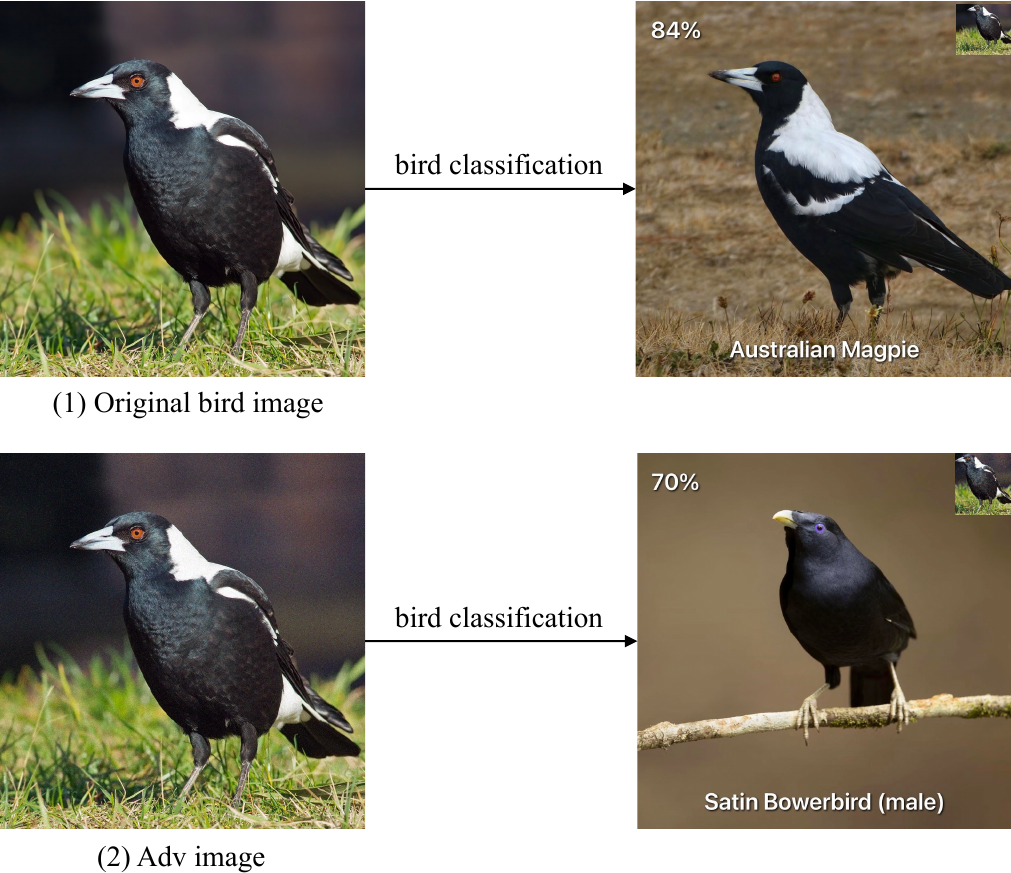}
    \caption{Example of attacking the feature of bird classification in the real-world app \emph{smart bird id}. The \emph{Adv image} is generated by attacking the corresponding model on Android}
    \label{fig:phAt2}
\end{figure}
